# Supplementary material for: Toward Agile Maneuvers in Highly Constrained Spaces: Learning from Hallucination
Source: arXiv:2007.14479 source file (2021-01-20)
Supplement: Supplementary file 1 [file supplementary.tex]

\section*{Appendix A: Quantifying the Complexity of Hallucination Space}
In this section we use a simple gridworld to illustrate the change in input space complexity, i.e. difference in domain size between $f(\cdot)$ and $g^{-1}(\cdot)$, when hallucination is used.
\begin{figure}[h]
    \centering
    \includegraphics[width=\textwidth]{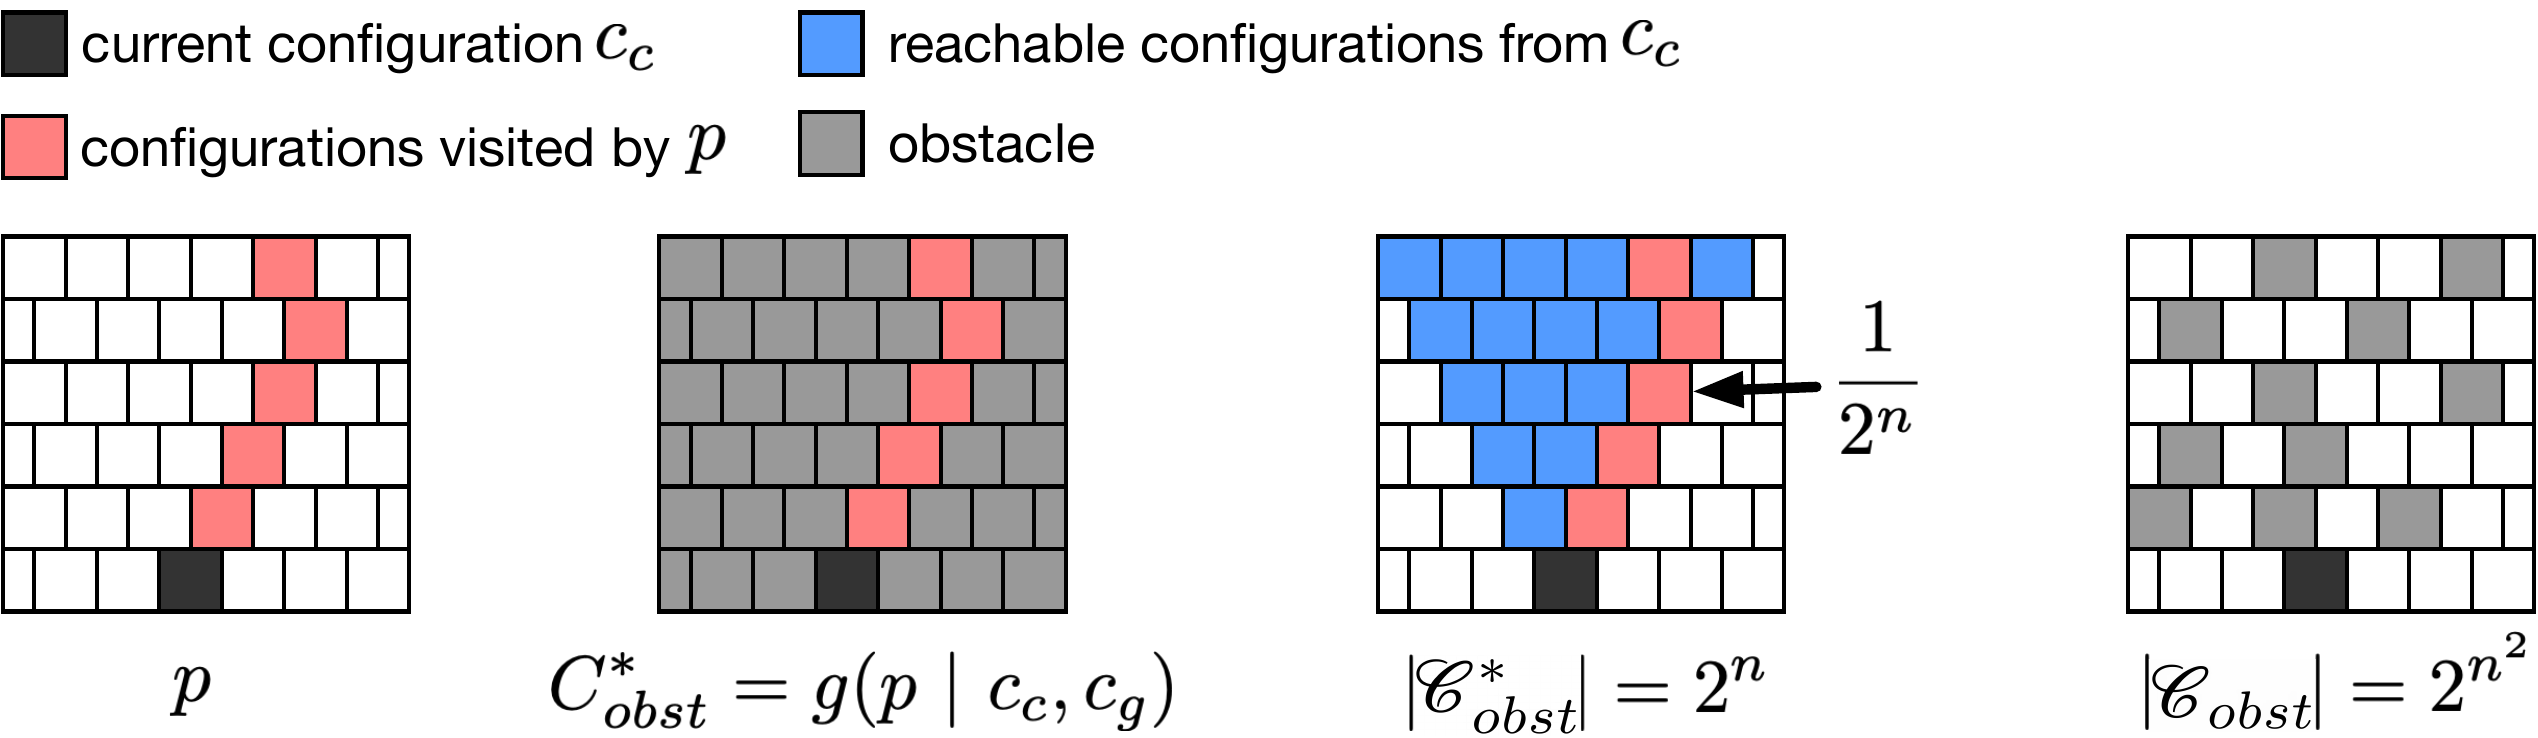}
    \caption{A simple gridworld to illustrate the complexity of hallucination space}
    \label{fig:complexity}
\end{figure}
\newline
Considering a 2D gridworld as shown in Figure~\ref{fig:complexity}, the agent is at the current configuration $c_c$ and at each step can visit the upleft or upright grid in front of it. The possible $C_{obst}$ configuration within the $n\times n$ gridworld in front the agent is $|\mathcal{C}_{obst}| = 2^{n^2}$, since for each grid, there either exists or not exists an obstacle. However, the hallucination space is essentially of the same complexity as the possible planning trajectories, because there exists a one-to-one relationship between a planning trajectory and its most constraint $C^*_{obst}$. The part of gridworld marked in blue are the reachable configurations from $c_c$, and there are in total $2^n$ possible planning trajectories, and therefore $2^n$ different $C^*_{obst}$. In general, if each time step the agent can go to $x$ nearby grids, then $|\mathcal{C}^*_{obst}| = x^n$. The main message here is the original configuration space is much larger than the hallucination space, i.e. $2^{n^2} = (2^n)^n$, where $n$ can be regarded as the planning horizon. This is the main cause of the data-efficiency and good generalization ability of the LfH method.

\section*{Appendix B: Implementation Details}

\subsection*{Pre-Processing}
\paragraph{Savitzky–Golay Filter}
The purpose of the Savitzky–Golay filter is to smooth the coarse global path so that it looks similar to the robot trajectory in the training set, with which the hallucinated training data is generated. The difference between the two can be caused by (1) highly discrete global path waypoints vs. high-resolution robot trajectory, (2) imperfections from \texttt{move\textunderscore base} global planner, e.g.jitters, irregularities, vs. smooth robot trajectory, and (3) two-dimensional ($x$, $y$) global waypoints without orientation vs. actual robot trajectory that fully observes nonholonomic constraints. 

To address the global planner's inability to consider nonholonomic constraints, we replace the first ten global waypoints with artificial waypoints, evenly distributed between the middle points of the rear and front bumper. The distribution of these artificial waypoints can be adjusted based on the hallucinated LiDAR's field-of-view. Then we apply Savitzky–Golay filter with $window\_length = 19, polyorder = 3 $. We empirically observe the filtered global path is similar to the robot trajectory in the training set. 

\paragraph{PID Controller }
The purpose of the PID controller is to drive the robot back from out-of-distribution scenarios unseen in the training set. One particular out-of-distribution scenario is when the planned global path leads to somewhere behind the robot. Instead of a U-turn with a smooth Dubin's path, the coarse global path directly connects the robot to somewhere behind. In such scenarios, we use the PID controller to rotate the robot in place, so that the difference between the current robot heading and the current tangential direction of the global path always falls in the range $[-30^{\circ}, 30^{\circ}]$. We empirically observe a proportional gain of $1$ suffices, while smoother turning can be enabled by adding integration and derivative parts. Paired with the Savitzky–Golay filter, any robot state within this $60^{\circ}$ range is in distribution of the training data.

\subsection*{Hallucination}
\paragraph{Hallucination Footprint}
The Jackal's half-width is 0.165m. During training, we use a hallucination footprint of 0.18m, i.e. any space further than 0.18m to the left and right hand side of the robot trajectory is hallucinated as occupied. In this way, a ``narrow corridor'' is built and we hallucinate the LiDAR input using raycasting.  

\paragraph{LiDAR Parameters}
A 2D LiDAR suffices for our LfH controller, We use ROS \texttt{pointcloud\textunderscore to\textunderscore laserscan} package to transfer the 3D Velodyne pointcloud to 2D laserscan. The 360$^{\circ}$ field-of-view ($angle\_min=-3.1415926$ and $angle\_max=3.1415926$) with $angle\_increment=0.003$ has 2095 laser beams and everything between the height $[0, 0.5]$m is treated as an obstacle. 

\paragraph{Network Architecture}
The LfH planner is a three-layer neural network, with 256 hidden neurons and ReLU activation for each layer. It takes in LiDAR input (normalized to $[-0.5, 0.5]$), current $v$ and $\omega$ (normalized to $[0, 1]$ and $[-1, 1]$, respectively), and $(x, y)$ coordiantes of the local goal. The output is one single action $u_1 = \{v_1, \omega_1\} \in p$. 

\paragraph{Training}
A snapshot of the collected training data is shown in Figure \ref{fig::trajectory_vw}. The green path in Figure \ref{fig::trajectory} represents the global $(x, y)$ trajectory of the robot, while the blue and red profiles in Figure \ref{fig::vw} represent the linear and angular velocity, $v$ and $\omega$, respectively. For each data point, we take its 100 neighbors to create the hallucination. Examples of the hallucinated training LiDAR data are displayed in Figure \ref{fig::lidar}. 

\begin{figure}
\centering
\subfloat[Robot Trajectory]{\includegraphics[width=0.4\columnwidth]{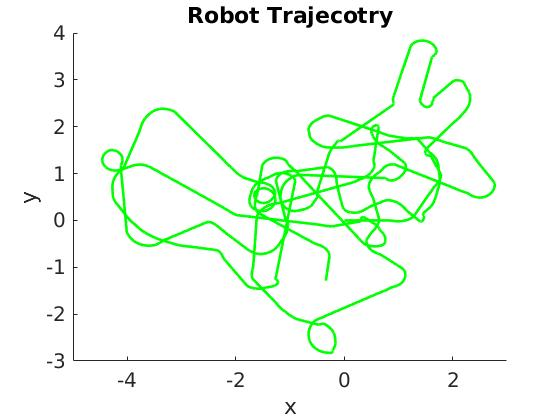}%
\label{fig::trajectory}}
\hspace{1pt}
\subfloat[Linear and Angular Velocities]{\includegraphics[width=0.4\columnwidth]{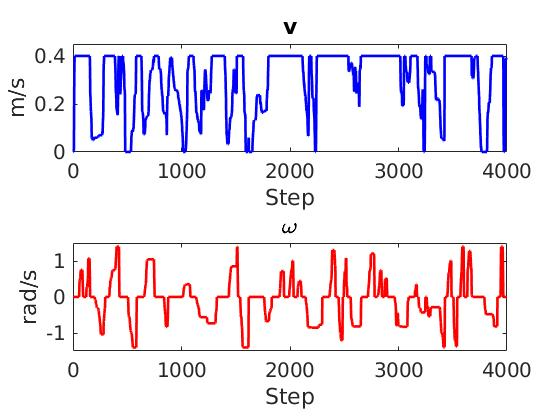}%
\label{fig::vw}}
\hspace{1pt}
\caption{Visualization of the Training Data}
\label{fig::trajectory_vw}
\end{figure}

\begin{figure}
\centering
\includegraphics[width=1\columnwidth]{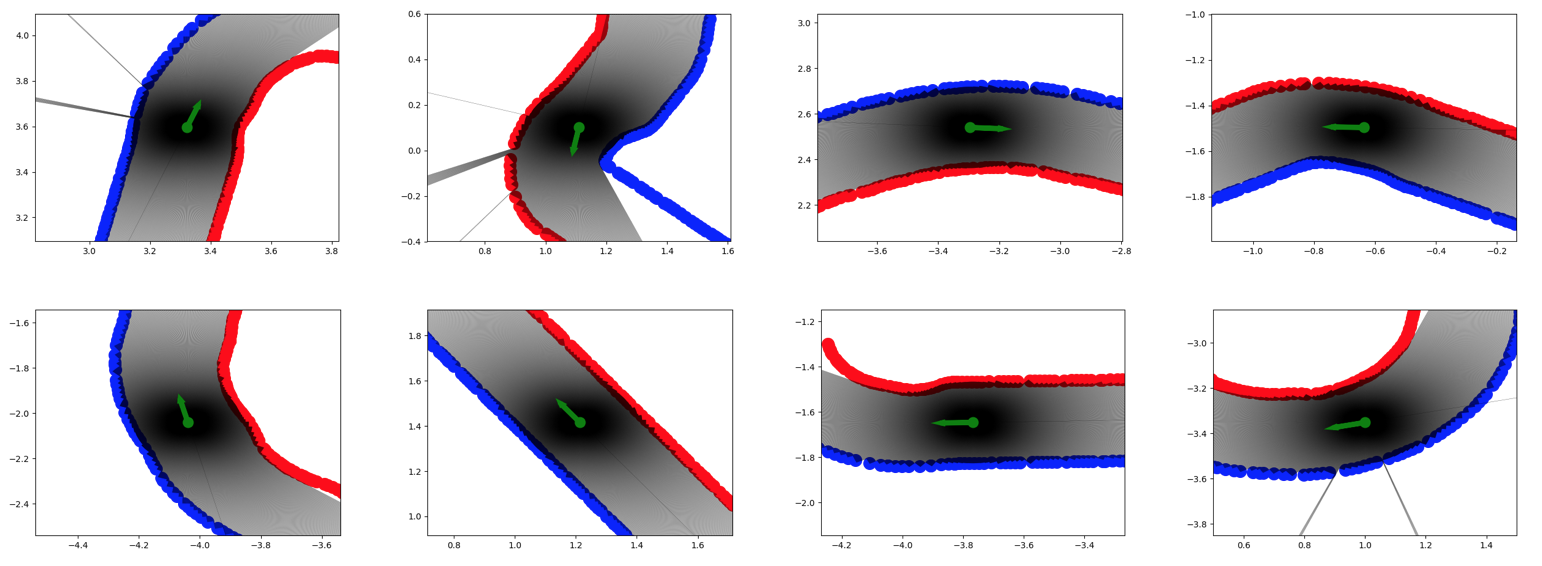}
\caption{Examples of Hallucinated Training LiDAR Data: Green dot represents the robot and green arrow is the orientation. Blue and red dots are the hallucinated obstacles on the left and right hand side of the robot trajectory, respectively. The black rays represent LiDAR beams. Some ``leaky'' LiDAR beams exist due to numerical error. }
\label{fig::lidar}
\end{figure}

\subsection*{Post-Processing}
\paragraph{Safety Estimation}
Gaussian noise of zero mean and 10\% standard deviation is added to the produced $v$ and $\omega$ for safety estimation. The MPC collision checker looks 20 steps ahead with 0.0625s integration interval on a batch size of 32 samples. For each sample, we check if any of the 40 points evenly distributed on the four edges of the vehicle after motion is further to the origin than the corresponding LiDAR beam reading. If any of them is, this sample causes a collision. We then compute the percentage of safe samples. 

\paragraph{Speed Modulation}
We modulate the controls with 
\[
e^{w_1-w_2(1-P(\text{safety}))}\cdot \{v, \omega\},
\]
where the weights for the speed modulation $w_1=0.4$ and $w_2=1.0$ correspond to roughly 50\% - 150\% modulation. In order to prevent noisy $\omega$ being amplified by the modulation in safe spaces, we suppress any $\omega < 0.04$rad/s to $0$.

\paragraph{Recovery Behavior}
When a predicted and modulated $\{v, \omega\}$ pair is not safe according to the MPC collision checker, the robot performs a three-stage recovery behavior. In the first stage, the robot iteratively decreases $v$ and increases $\omega$, both by 2\%, until the resulted $\{v, \omega\}$ is safe. If it is still not safe after 20 iterations, the robot enters the second stage. It negates $v$, and increases both negated $v$ and original $\omega$ by 2\% in each step. If this is still not safe after 20 more iterations, the robot backs up at 0.1m/s in stage three. 

\section*{Appendix C: Experiment Details}
\subsection*{DWA}
ROS \texttt{move\textunderscore base} navigation stack's default local planner, DWA, is used as our first baseline. We use the default parameters recommended by the robot manufacturer, Clearpath Robotics. The specific values of the parameters are shown in the second row of Table \ref{tab::jackal_parameters}. 

\subsection*{Behavior Cloning}
We use the same neural network architecture as LfH, but with realistic in stead of hallucinated LiDAR input. The experienced human demonstrator aims at tele-operating the robot to traverse through the obstacle course in a fast and safe manner. The entire demonstration lasts 67.8s. 

\subsection*{APPLD}
Using the same 67.8s demonstration, APPLD first automatically segments the demonstration into four contexts. Within each context, we use a black-box optimization technique, CMA-ES, to tune the optimal set of DWA parameters that imitate the human demonstration. The resulted values of the four sets of parameters after eight hours of training are shown in the last four rows of Table \ref{tab::jackal_parameters}. The robot switches among these four sets of parameters using the prediction of a LiDAR-based context predictor (a neural network with one hidden layer of ten neurons).

\begin{table}
\centering
  \caption{Parameter Values Used by Default DWA and APPLD: \emph{max\_vel\_x } \textnormal{(v)}, \emph{max\_vel\_theta} \textnormal{(w)}, \emph{vx\_samples} \textnormal{(s)}, \emph{vtheta\_samples} \textnormal{(t)}, \emph{occdist\_scale} \textnormal{(o)}, \emph{pdist\_scale} \textnormal{(p)}, \emph{gdist\_scale} \textnormal{(g)}}
%   \vspace{-5pt}
  \label{tab::jackal_parameters}
  \centering
  \small
  \begin{tabular}{lrrrrrrr}
    \toprule
                & v & w & s & t & o & p & g \\
    \midrule
    Default         & 0.50 & 1.57 &  6 & 20 & 0.10 & 0.75 & 1.00\\
    \midrule
    Context 1       & 0.40 & 0.85 & 17 & 15 & 0.69 & 0.96 & 0.75\\
    Context 2       & 0.35 & 1.52 & 16 & 15 & 0.92 & 0.69 & 0.43\\
    Context 3       & 0.42 & 2.18 & 13 & 19 & 0.76 & 0.06 & 0.39\\
    Context 4       & 0.25 & 1.34 & 8 & 40 & 0.43 & 0.65 & 0.98\\
    \bottomrule
  \end{tabular}
\end{table}

\newpage
